# Supplementary material for: A Vanilla Multi-Task Framework for Dense Visual Prediction Solution to 1st VCL Challenge -- Multi-Task Robustness Track
Source: arXiv:2402.17319 source file (2024-02-27)
Supplement: Supplementary file 1 [file appendix.tex]

\appendix

\section{Results on Waymo Dataset}

\section{Extension to 2D Object Detection}
